# Supplementary material for: Pathway-Structured Privileged Distillation for Deployable Computational Pathology
Source: arXiv:2606.02877 source file (2026-10-16)
Supplement: Supplementary file 1 [file sn-supplementary-information.tex]

\documentclass[pdflatex,sn-nature]{sn-jnl}
\usepackage{amsmath,amssymb}
\usepackage{textcomp}

\begin{document}

\title[Supplementary Information]{Supplementary Information for Pathway-Structured Privileged Distillation for
Deployable Computational Pathology}
\maketitle

\section*{Supplementary Note 1: Clinical and Biological Context of Classification Tasks}

\subsection*{1. Oncotype DX (ODX) Risk Status in Breast Cancer (TCGA-BRCA)}
The Oncotype DX assay is a widely adopted 21-gene expression signature used to quantify the risk of distant recurrence in patients with early-stage, estrogen receptor-positive (ER+), and HER2-negative breast cancer. Clinically, it can inform adjuvant treatment decisions. Because the genomic assay requires additional tissue, cost and turnaround time, predicting ODX risk status from routine H\&E-stained whole-slide images (WSIs) provides a clinically motivated benchmark for WSI-only risk prediction.

\subsection*{2. Progesterone Receptor (PR) Status in Breast Cancer (TCGA-BRCA)}
Progesterone receptor (PR) is a nuclear hormone receptor whose expression is a fundamental prognostic and predictive biomarker in breast cancer. PR positivity is often associated with more differentiated, endocrine-responsive disease. Inferring PR status from histopathology morphology provides a benchmark for testing whether the model captures predictive information associated with molecularly linked phenotypic patterns.

\subsection*{3. Hypoxia Status in Lung Adenocarcinoma (TCGA-LUAD)}
Tumour hypoxia is a hallmark of the solid tumour microenvironment, characterized by oxygen deprivation that triggers the Hypoxia-Inducible Factor (HIF) signalling pathways. Biologically, hypoxia is associated with angiogenesis, metabolic reprogramming and aggressive metastasis. Clinically, it is associated with poor prognosis and resistance to both radiotherapy and chemotherapy. Predicting hypoxia-related labels from WSIs tests whether morphological alterations, such as microvascular abnormalities or necrosis, contain information associated with hypoxic tumour states.

\subsection*{4. Epidermal Growth Factor Receptor (EGFR) Status in Lung Adenocarcinoma (TCGA-LUAD)}
Mutations in the Epidermal Growth Factor Receptor (EGFR) gene are among the most common actionable driver alterations in non-small cell lung cancer (NSCLC), predominantly occurring in lung adenocarcinoma. Patients harboring sensitizing EGFR mutations can respond to targeted EGFR tyrosine kinase inhibitors (TKIs). However, conventional molecular profiling, such as next-generation sequencing, can be delayed by tissue constraints and lengthy turnaround times. Predicting EGFR status through computational pathology therefore provides a clinically motivated benchmark for assessing whether WSIs contain predictive information associated with EGFR status.

\subsection*{5. Mesenchymal State in Glioma (TCGA-GBMLGG)}
Glioblastoma and lower-grade gliomas can be classified into distinct transcriptional subtypes, among which the mesenchymal state is aggressive. This subtype is characterized by neuro-inflammation, angiogenesis, macrophage infiltration and resistance to standard chemo-radiation therapies. Predicting the mesenchymal state from H\&E slides provides a benchmark for testing whether morphology contains predictive information associated with transcriptional glioma state.

\section*{Supplementary Note 2: Pathway observability analysis using Cohen's \texorpdfstring{$d$}{d}}

We used Cohen's \(d\) to quantify pathway-level separation between task-defined groups. For each Hallmark pathway \(p\), the RNA-side relevance was computed from RNA-derived pathway scores, whereas WSI-side gate separation was computed from the gate values of the corresponding WSI pathway expert. This allowed molecular pathway relevance and histology-side model-usage patterns to be compared on the same standardized effect-size scale.

For the RNA-side analysis, each patient had a precomputed RNA-derived pathway matrix. Let \(G_p\) denote the set of genes or pathway features assigned to Hallmark pathway \(p\). For patient \(i\), the RNA-side pathway score was computed by averaging the corresponding RNA-derived values over the features belonging to that pathway:
\[
S^{\mathrm{RNA}}_{i,p}
=
\frac{1}{|G_p|}
\sum_{g \in G_p}
M_{i,p,g},
\]
where \(M_{i,p,g}\) denotes the RNA-derived value for patient \(i\), pathway \(p\) and feature \(g\). Thus, each patient received one RNA-side score for each of the 50 Hallmark pathways.

For the WSI-side analysis, we used the expert gate vector produced by the WSI branch. For slide \(i\), let
\[
S^{\mathrm{WSI}}_{i,p}=g_{i,p}
\]
denote the gate value assigned to pathway expert \(p\). Thus, the RNA-side axis measures separation in RNA-derived pathway scores, whereas the WSI-side axis measures separation in learned WSI expert usage.

For each pathway \(p\), samples were divided into task-defined positive and negative groups. In the BRCA-ODX analysis, the positive group corresponded to ODX-high cases and the negative group corresponded to ODX-low cases. Let \(x_{p,i}^{+}\) denote the value for sample \(i\) in the positive group and \(x_{p,j}^{-}\) denote the value for sample \(j\) in the negative group. Depending on the axis, \(x\) represents either the RNA-derived pathway score \(S^{\mathrm{RNA}}_{i,p}\) or the WSI expert gate value \(S^{\mathrm{WSI}}_{i,p}\). If the two groups contain \(n_{+}\) and \(n_{-}\) samples, their group means are
\[
\mu_{p}^{+}=\frac{1}{n_{+}}\sum_{i=1}^{n_{+}}x_{p,i}^{+},
\qquad
\mu_{p}^{-}=\frac{1}{n_{-}}\sum_{j=1}^{n_{-}}x_{p,j}^{-}.
\]

The corresponding sample variances are
\[
(s_{p}^{+})^{2}
=
\frac{1}{n_{+}-1}
\sum_{i=1}^{n_{+}}
\left(x_{p,i}^{+}-\mu_{p}^{+}\right)^2,
\qquad
(s_{p}^{-})^{2}
=
\frac{1}{n_{-}-1}
\sum_{j=1}^{n_{-}}
\left(x_{p,j}^{-}-\mu_{p}^{-}\right)^2.
\]

The pooled standard deviation is
\[
s_{p,\mathrm{pooled}} =
\sqrt{
\frac{
(n_{+}-1)(s_{p}^{+})^{2}
+
(n_{-}-1)(s_{p}^{-})^{2}
}
{n_{+}+n_{-}-2}
}.
\]

Cohen's \(d\) for pathway \(p\) is then
\[
d_p =
\frac{\mu_{p}^{+}-\mu_{p}^{-}}
{s_{p,\mathrm{pooled}}}.
\]

In the pathway observability analysis, we used the absolute value,
\[
|d_p|,
\]
because the goal was to measure the magnitude of pathway separation rather than the direction of association. A larger \(|d_p|\) therefore indicates stronger separation between the task-defined groups.

For the BRCA-ODX observability map, the horizontal coordinate of pathway \(p\) was
\[
x_p = |d^{\mathrm{RNA}}_p|,
\]
computed from RNA-derived pathway scores in the paired BRCA-ODX cohort. The vertical coordinate was
\[
y_p = |d^{\mathrm{WSI}}_p|,
\]
computed from the WSI pathway expert gate values for the same prediction task. Each point therefore represents one Hallmark pathway, with its horizontal position indicating RNA-side pathway relevance and its vertical position indicating WSI-side gate separation.

For the external ODX cohort, transcriptomic profiles were unavailable. We therefore used the RNA-side \(|d^{\mathrm{RNA}}_p|\) values estimated from the paired BRCA-ODX cohort as a fixed transcriptomic reference, and recomputed the WSI-side \(|d^{\mathrm{WSI}}_p|\) values using expert gate values from the external WSI cohort. This design compares external WSI-side gate separation with an internal RNA-side reference, without claiming direct external RNA-side validation.

Point colour represents the top-3 expert frequency for each pathway expert. For each WSI sample, we identified the three pathway experts with the largest gate values. The top-3 frequency of expert \(p\) was computed as the fraction of samples in which expert \(p\) appeared among these three highest-gated experts. Thus, point position summarizes group-separation effect size, whereas point colour summarizes how frequently the WSI model actively selected that pathway expert.

The resulting comparison maps were used to define four descriptive regimes using median thresholds over the 50 Hallmark pathways on each axis: RNA-relevant and higher WSI-side gate-separation pathways, RNA-relevant but weak WSI-side gate-separation pathways, morphology-associated proxy programmes and weak or low-relevance pathways. These regimes are intended as descriptive summaries of model-usage patterns and should not be interpreted as direct evidence of pathway activation or causal pathway regulation.

For the omics-only comparison in the main text, we used GPNet as an independent RNA-side reference model. MoPE pathway scores were computed from the mean WSI expert-gate values for each Hallmark pathway. GPNet pathway scores were computed from pathway-level association statistics after Benjamini--Hochberg correction. Scores were normalized within each model to form pathway-score profiles, allowing pathways to be ranked and compared across the WSI and omics-only models. For a given \(k\), the top-\(k\) overlap was computed as the fraction of the top \(k\) pathways shared by the two ranked lists; the random expectation is \(k/50\) for 50 Hallmark pathways. This comparison is descriptive and should not be interpreted as external validation of molecular pathway activity.

\section*{Supplementary Note 3: Structured prompt for large language model-assisted morphology summarization}

In this work, a large language model was used to convert model-derived visual evidence into a standardized morphology summary for subsequent clinical expert review. The model provider, model version and access date must be confirmed by the authors before submission. The prompt used internal input panels, which are referred to below as Prompt Panels A--E to avoid confusion with the main-text figures.

\begin{quote}
Act as a senior computational pathologist and molecular biologist. Your task is to interpret model-selected H\&E regions from a pathway-aware multi-slot WSI model using standard pathology terminology. Do not make a definitive diagnosis and do not claim molecular pathway activation from morphology alone.

\textbf{Cancer and model context.} Cancer type: BRCA invasive breast carcinoma. Task: ODX risk prediction. Each expert corresponds to one Hallmark pathway, and multiple slots under the same expert are trained to capture different visual morphology patterns. The goal is to interpret whether the slots collectively provide complementary visual evidence for the same pathway-level biological process. Selected expert: Expert 17. Corresponding Hallmark pathway: G2M\_Checkpoint. Selected top slots: the high-gated slots shown in Prompt Panels B--E.

\textbf{Input panels.} Prompt Panel A shows the original WSI and top expert-level heatmaps. Prompt Panel B shows slot-level heatmaps for the selected expert. Prompt Panels C--E show top high-attention H\&E patch tiles for the top three slots of the selected expert.

\textbf{Interpretation principles.} First describe visual evidence and then discuss biological consistency. Use standard pathology terminology. Do not infer pathway activation. Use cautious language such as ``morphologically compatible with'', ``may reflect'' or ``could be consistent with''. Do not penalize slots for being morphologically different, and do not treat one slot as sufficient evidence for the whole pathway. If the morphology is nonspecific, mixed or low resolution, state this explicitly. Hallmark gene sets are transcriptional biological programmes, not official histological morphology categories; morphology can only support compatibility with a pathway, not prove pathway activation.

\textbf{Analysis tasks.} Describe expert-level spatial attention; compare slot-level spatial patterns; describe patch morphology for each selected slot, including architecture, cytology, microenvironment and a concise slot morphology concept; synthesize cross-slot similarities and differences; rate consistency with the provided Hallmark pathway as strong, moderate, weak or not supported; and write a 2--4 sentence manuscript-style summary.

\textbf{Required output.} Provide cancer and model context, expert-level spatial attention, slot-level analysis for each selected slot, cross-slot synthesis, Hallmark pathway consistency, alternative interpretations, limitations and a manuscript-style summary.
\end{quote}

\end{document}
